# Supplementary material for: IPPON: Common Sense Guided Informative Path Planning for Object Goal Navigation
Source: arXiv:2410.19697 source file (2024-10-25)
Supplement: Supplementary file 1 [file appendix.tex]

\section{LLM Prompt and Example Responses}

The prompt used for querying the LLM about object proximity is detailed in Listing~\ref{lst:llm_prompt}. It includes placeholders \texttt{\{ooi\}}, \texttt{\{common\_objects\}}, \texttt{\{scenario\}}, and \texttt{\{context\_information\}}, which are described as follows:

For the Habitat ObjectNav Challenge 2023:
\begin{itemize}
    \item Options for \texttt{\{ooi\}}: chair, bed, plant, toilet, tv, sofa.
    \item \texttt{\{common\_objects\}}: wall, floor, chair, door, table, picture, cabinet, cushion, window, sofa, bed, curtain, chest of drawers, plant, sink, stairs, ceiling, toilet, stool, towel, mirror, tv, shower, column, bathtub, counter, fireplace, lighting, beam, railing, shelving, blinds, gym equipment, seating, board panel, furniture, appliances, clothes, objects, others.
    \item \texttt{\{scenario\}}: an apartment with different rooms.
    \item \texttt{\{context\_information\}}: Not applicable.
\end{itemize}

For hardware experiments in the lab:
\begin{itemize}
    \item Options for \texttt{\{ooi\}}:
        \begin{itemize}
            \item Basic categories: plant, chair, tv, sofa.
            \item Open-vocabulary categories: toy elephant, screwdriver, microwave oven, coffee machine.
            \item Context-specific categories: hat, student card.
            \item Outdoor categories: plant, ping pong table, ping pong paddles.
        \end{itemize}
    \item \texttt{\{common\_objects\}}: wall, floor, stairs, ceiling, railing, window, lighting, shelving, sink, door, chair, table, counter, chest of drawers, sofa, metal cabinet, kitchen cabinet, plant, tv, monitor, computer, poster, whiteboard, coat rack, trash can, fire extinguisher, toolbox, cart, robot, crane, charger, fridge, printer, microwave oven, coffee machine, dishwasher, equipment, phone booth, ping pong table, others.
    \item \texttt{\{scenario\}}: a robotics lab.
    \item \texttt{\{context\_information\}}:
        \begin{itemize}
            \item Hat: He just called me and said, ``I think I forgot my hat on the sofa. I left it there yesterday when I was taking a nap.''
            \item Student card: He just called me and said, ``I just use it on the printer.''
        \end{itemize}
\end{itemize}

\begin{lstlisting}[captionpos=t, caption={Prompt for querying object proximity levels.}, label={lst:llm_prompt}]
I am an assistant autonomous robot trying to help my owner find a {ooi} (object). {context_information}.

My search is within {scenario}, which has the following list of common categories: {common_objects}.

Now I need your help to search for objects more efficiently. For each category, please assign its proximity level to a {ooi}, indicating how likely it is to find a {ooi} nearby if I am close to that category. The proximity level should be only based on the horizontal distance between the categories, and the vertical distance should be ignored as I can look up and down freely. Here's an explanation of different proximity levels.

- FAR: The presence of such a category suggests that the {ooi} is located somewhere far away (e.g., in another room). For example, if I see a sink, it is unlikely that I will find a bed nearby because sink is usually placed in the kitchen or bathroom.

- AVERAGE: There is no significant indication whether a {ooi} is typically located near or far away from this category. Please ensure all pervasive elements like walls, floors, ceilings, and doors fall into this level as they are almost everywhere and don't provide much information. Moreover, please also ensure that all broad categories that contain {ooi} but also others are rated as AVERAGE because they are too general to provide any useful information. This is the most common proximity level and should be considered as the default unless there is a strong indication.

- NEAR: A {ooi} is typically found near this category. For example, if I am close to bed or sofa, then it is likely that I will find a TV nearby.

- CERTAIN: It is certain that the {ooi} is in the vicinity, or the category directly corresponds to the object I am searching for (as my owner only needs to find one instance).

Note the asymmetry in object proximity: finding A when close to B is not the same as finding B when close to A. For instance, the presence of the floor is nearly guaranteed (CERTAIN) when I am close to a chair because chairs are typically placed on floors. However, the reverse scenario - finding a chair when I am close to the floor - should be rated as AVERAGE because floors cover large areas (pervasive elements), and chairs can be placed anywhere.

Please use your common sense and justify your ratings before you provide the proximity level. Strictly follow this format: '[category]: [explanation]. [FAR/AVERAGE/NEAR/CERTAIN]'. Stick to the plain text format without any extra formatting. Do not change the category name in any way because I will be retrieving them using regular expressions.
\end{lstlisting}

We provide two examples of the proximity levels in Listing~\ref{lst:bed-proximity} and \ref{lst:sofa-promixity-levels}. Listing~\ref{lst:bed-proximity} shows the proximity levels between a chair and common objects in the Habitat ObjectNav 2023 Challenge, which relates to the episode depicted in Figures \ref{fig:ippon-pipeline} and \ref{fig:imagined-probability}. The other example involves finding a hat in the lab, given the context, ``I think I forgot my hat on the sofa. I left it there yesterday when I was taking a nap.'' Note that the object proximity levels can be saved and reloaded if the OOI and common objects have already been queried.

\begin{lstlisting}[captionpos=t, caption={Proximity levels between a bed and common objects in the Habitat ObjectNav Challenge.}, label={lst:bed-proximity}]
appliances:
  explanation: Appliances are typically found in kitchens or bathrooms, not near a bed
  proximity: FAR
bathtub:
  explanation: Bathtubs are found in bathrooms, not near a bed
  proximity: FAR
beam:
  explanation: Beams can be found in various parts of a home and don't indicate a bed nearby
  proximity: AVERAGE
bed:
  explanation: This is the object you're searching for, so its presence guarantees a bed is nearby
  proximity: CERTAIN
blinds:
  explanation: Blinds can be found in any room with windows, including bedrooms
  proximity: AVERAGE
board_panel:
  explanation: Board panels can be found in various parts of a home and don't indicate a bed nearby
  proximity: AVERAGE
cabinet:
  explanation: Cabinets are usually found in kitchens or bathrooms, not typically near a bed
  proximity: FAR
ceiling:
  explanation: Ceilings are pervasive elements and can be found in every room, including bedrooms
  proximity: AVERAGE
chair:
  explanation: Chairs can be found in various rooms, not necessarily near a bed
  proximity: AVERAGE
chest_of_drawers:
  explanation: Chests of drawers are often found in bedrooms, so there's a good chance a bed is nearby
  proximity: NEAR
clothes:
  explanation: Clothes can be found in various rooms, including bedrooms, so there's a chance a bed could be nearby
  proximity: NEAR
column:
  explanation: Columns can be found in various parts of a home and don't indicate a bed nearby
  proximity: AVERAGE
counter:
  explanation: Counters are typically found in kitchens or bathrooms, not near a bed
  proximity: FAR
curtain:
  explanation: Curtains can be found in any room with windows, including bedrooms
  proximity: AVERAGE
cushion:
  explanation: Cushions can be found on sofas or beds, so there's a chance a bed could be nearby
  proximity: NEAR
door:
  explanation: Doors are pervasive elements and can be found in every room, including bedrooms
  proximity: AVERAGE
fireplace:
  explanation: Fireplaces are typically found in living rooms, not near a bed
  proximity: FAR
floor:
  explanation: Floors are also pervasive elements and can be found in every room, including bedrooms
  proximity: AVERAGE
furniture:
  explanation: Furniture is a broad category that includes beds, so its presence doesn't necessarily indicate a bed nearby
  proximity: AVERAGE
gym_equipment:
  explanation: Gym equipment is typically not found near a bed
  proximity: FAR
lighting:
  explanation: Lighting is a pervasive element and can be found in every room, including bedrooms
  proximity: AVERAGE
mirror:
  explanation: Mirrors can be found in various rooms, including bedrooms, so there's a chance a bed could be nearby
  proximity: NEAR
objects:
  explanation: Objects is a broad category that doesn't provide specific information about a bed's location
  proximity: AVERAGE
others:
  explanation: Others is a broad category that doesn't provide specific information about a bed's location
  proximity: AVERAGE
picture:
  explanation: Pictures can be hung in any room, including bedrooms, but their presence doesn't necessarily indicate a bed nearby
  proximity: AVERAGE
plant:
  explanation: Plants can be placed in any room, including bedrooms, but their presence doesn't necessarily indicate a bed nearby
  proximity: AVERAGE
railing:
  explanation: Railings are typically found on stairs or balconies, not near a bed
  proximity: FAR
seating:
  explanation: Seating can be found in various rooms, not necessarily near a bed
  proximity: AVERAGE
shelving:
  explanation: Shelving can be found in various rooms, not necessarily near a bed
  proximity: AVERAGE
shower:
  explanation: Showers are found in bathrooms, not near a bed
  proximity: FAR
sink:
  explanation: Sinks are typically found in kitchens or bathrooms, not near a bed
  proximity: FAR
sofa:
  explanation: Sofas are typically found in living rooms, not bedrooms. However, in some studio apartments, a bed might be near a sofa
  proximity: AVERAGE
stairs:
  explanation: Stairs lead to different levels of a home and don't indicate a bed nearby
  proximity: FAR
stool:
  explanation: Stools can be found in various rooms, not necessarily near a bed
  proximity: AVERAGE
table:
  explanation: Tables can be found in various rooms, not necessarily near a bed
  proximity: AVERAGE
toilet:
  explanation: Toilets are found in bathrooms, not near a bed
  proximity: FAR
towel:
  explanation: Towels are typically found in bathrooms or kitchens, not near a bed
  proximity: FAR
tv:
  explanation: TVs can be found in living rooms or bedrooms, so there's a chance a bed could be nearby
  proximity: NEAR
wall:
  explanation: Walls are pervasive elements in an apartment and can be found in every room, including bedrooms
  proximity: AVERAGE
window:
  explanation: Windows are pervasive elements and can be found in every room, including bedrooms
  proximity: AVERAGE
\end{lstlisting}

\begin{lstlisting}[captionpos=t, caption={Proximity levels between a hat and common objects in the lab, with context provided.}, label={lst:sofa-promixity-levels}]
cart:
  explanation: Carts could be used in various settings, but they do not specifically
    indicate the proximity to a hat
  proximity: AVERAGE
ceiling:
  explanation: Ceilings cover every room but do not provide information on the
    location of a hat
  proximity: AVERAGE
chair:
  explanation: Chairs could be near places where someone might take off a hat,
    but they are not a strong indicator on their own
  proximity: AVERAGE
charger:
  explanation: Chargers are for recharging batteries and do not indicate the proximity
    to a hat
  proximity: FAR
chest_of_drawers:
  explanation: A chest of drawers might be a place where a hat is stored, but
    without specific information, it's not a strong indicator
  proximity: AVERAGE
coat_rack:
  explanation: A coat rack could be a place where hats are hung, making it a possible
    location to find a hat
  proximity: NEAR
coffee_machine:
  explanation: Coffee machines are found in kitchen or office settings, not indicating
    a hat's location
  proximity: FAR
computer:
  explanation: Computers, like monitors, are found in work areas, not typically
    where someone would leave a hat
  proximity: FAR
counter:
  explanation: Counters are common in kitchens and sometimes in other work areas,
    not specifically indicating a hat's location
  proximity: AVERAGE
crane:
  explanation: Cranes are used for lifting heavy items and do not relate to where
    a hat might be found
  proximity: FAR
dishwasher:
  explanation: Dishwashers are used for cleaning dishes, not related to where
    a hat might be found
  proximity: FAR
door:
  explanation: Doors are present in nearly all indoor environments, making them
    too general to indicate the proximity to a hat
  proximity: AVERAGE
equipment:
  explanation: Equipment is a broad category and could include anything from office
    to lab equipment, not specifically indicating a hat's location
  proximity: AVERAGE
fire_extinguisher:
  explanation: Fire extinguishers are safety equipment, not related to the storage
    or placement of personal items like hats
  proximity: FAR
floor:
  explanation: Floors are present everywhere within an indoor environment, thus
    not offering a clue towards the location of a hat
  proximity: AVERAGE
fridge:
  explanation: Fridges are unlikely places to find a hat, as they are used for
    storing food
  proximity: FAR
kitchen_cabinet:
  explanation: Kitchen cabinets are unlikely places to find a hat as they are
    used for storing kitchenware
  proximity: FAR
lighting:
  explanation: Lighting is a general feature of all indoor spaces and does not
    indicate the proximity to a hat
  proximity: AVERAGE
metal_cabinet:
  explanation: Metal cabinets are more likely used for storing tools or documents
    rather than hats
  proximity: FAR
microwave_oven:
  explanation: Microwave ovens are used for heating food and do not indicate the
    proximity to a hat
  proximity: FAR
monitor:
  explanation: Monitors are typically found in work or computer areas, which do
    not directly relate to where a hat might be found
  proximity: FAR
others:
  explanation: This is too general a category to provide any useful information
    regarding the proximity to a hat
  proximity: AVERAGE
phone_booth:
  explanation: Phone booths are rare and not indicative of the proximity to a
    hat in a modern setting
  proximity: FAR
ping_pong_table:
  explanation: Ping pong tables are used for recreation and do not specifically
    indicate the proximity to a hat
  proximity: FAR
plant:
  explanation: Plants are decorative and do not indicate the proximity to a hat
  proximity: FAR
poster:
  explanation: Posters are decorative and do not indicate the proximity to a hat
  proximity: FAR
printer:
  explanation: Printers are office equipment, not related to where a hat might
    be found
  proximity: FAR
railing:
  explanation: Railings are typically found near stairs or balconies, neither
    of which directly indicates the proximity to a hat
  proximity: AVERAGE
robot:
  explanation: Robots in a lab setting do not directly indicate the proximity
    to a hat
  proximity: FAR
shelving:
  explanation: Shelving could store a variety of items, including a hat, but it's
    not a direct indicator unless the hat is specifically known to be stored there
  proximity: AVERAGE
sink:
  explanation: Sinks are usually found in kitchens or bathrooms, places where
    hats are less likely to be left
  proximity: FAR
sofa:
  explanation: Given the owner's statement, the sofa is the specific location
    where the hat was left
  proximity: CERTAIN
stairs:
  explanation: Stairs connect different levels of a building but do not offer
    a specific indication of where a hat might be found
  proximity: AVERAGE
table:
  explanation: Tables are common in many rooms and could be places where hats
    are temporarily placed, but they do not strongly indicate the proximity to
    a hat
  proximity: AVERAGE
toolbox:
  explanation: Toolboxes are for storing tools, not typically a place where a
    hat would be found
  proximity: FAR
trash_can:
  explanation: Trash cans are not a likely place to intentionally leave a hat,
    providing no specific indication of a hat's proximity
  proximity: FAR
tv:
  explanation: TVs are common in living areas where someone might take off a hat,
    but they are not a direct indicator of a hat's location
  proximity: AVERAGE
wall:
  explanation: Walls are pervasive elements in any indoor environment, providing
    no specific indication of the proximity to a hat
  proximity: AVERAGE
whiteboard:
  explanation: Whiteboards are used in work or educational settings, not directly
    indicating a hat's location
  proximity: FAR
window:
  explanation: Windows are common in many rooms and do not offer a specific clue
    towards finding a hat
  proximity: AVERAGE

\end{lstlisting}

\section{Traversability Estimation}

The collision body of the robot is approximated by a list of collision spheres, consisting of base spheres $(\boldsymbol{c}_{base}(n), r_{base})$ that ensure ground contact, and body spheres $(\boldsymbol{c}_{body}(n), r_{body})$ that avoid collisions. Here, $\boldsymbol{c}$ and $r$ denote the center and radius of each collision sphere, respectively. We can write the traversability estimation as
\begin{equation}
    n \text{ untraversable} \; \iff \; sdf(\boldsymbol{c}_{base}(n)) \geq r_{base} \; \vee\; sdf(\boldsymbol{c}_{body}(n)) < r_{body},
    \label{eq:optimistic-traversability-estimation}
\end{equation}
where $sdf(\cdot)$ denotes the Euclidean signed distance field, calculated using Voxblox~\cite{oleynikova2017voxblox}. Fig.~\ref{fig:local-planning} illustrates the collision spheres for a legged robot with an arm and the Stretch robot used in the Habitat Challenge 2023.
\begin{figure}[ht]
    \centering
    \includegraphics[width=0.30\linewidth]{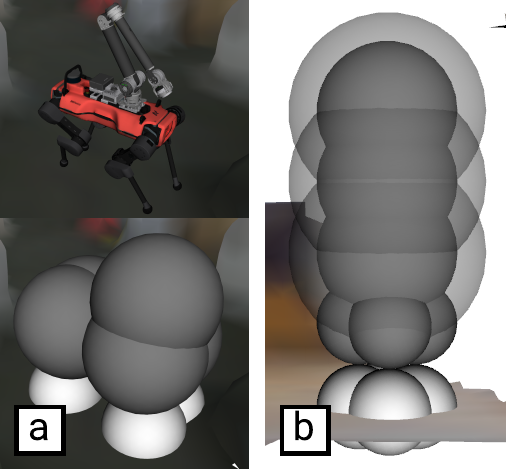}
    \caption{Collision spheres for a legged robot with an arm \textbf{(a)} and Stretch \textbf{(b)}. Habitat ObjectNav Challenge treats the Stretch robot as a cylindrical robot, standing 1.41 meters tall with a radius of 0.17 meters. The body is approximated with solid gray spheres and the base with white ones. The clearance (see Sec.~\ref{subsubsec:node-connecction}) is colored with transparent gray.}
    \label{fig:local-planning}
\end{figure}

Note that this approach is collision-optimistic, meaning any pose not explicitly identified as untraversable is assumed to be traversable. This strategy is necessary due to the robot's significant height and the common occurrence of occlusions, which makes it challenging to obtain complete $sdf$ for all spheres to properly evaluate traversability. For the ablation study, we removed clearance as a soft constraint and included it in the base collision spheres as a hard constraint (w/o clearance in Table~\ref{tab:ablations-object}).

% we check collision avoidance for the body and ensure contacts for the base, namely,
% \begin{equation}
%     sdf(\boldsymbol{c}_{body}(n)) \geq r_{body} \; \wedge\; sdf(\boldsymbol{c}_{base}(n)) < r_{base} \; \Longrightarrow \; n \text{ traversable} 
%     \label{eq:strict-traversability-estimation}
% \end{equation}
%  Since the robot doesn't possess prior map knowledge in the object goal navigation, $sdf(\cdot)$ could return a real value or unknown. The planner could be optimistic in estimating traversability, assuming $n$ is traversable unless a collision is confirmed to fail, as expressed by. 

\section{Additional Results}

We illustrate the effectiveness of semantic guidance in the Habitat ObjectNav 2023 Challenge in Fig.~\ref{fig:find-bed}. Furthermore, Fig.~\ref{fig:find-all-objects-proximity-map}  demonstrates the planner's ability to leverage a common object map from previous runs to efficiently localize new OOIs in real-world experiments. Additionally, Fig.~\ref{fig:find-microwave-oven-long-distance} highlights the planner's capability to find objects in challenging environments, where the robot must traverse long distances and navigate through multiple turns to reach the OOI.

\begin{figure}[ht]
    \centering
    \includegraphics[width=\linewidth]{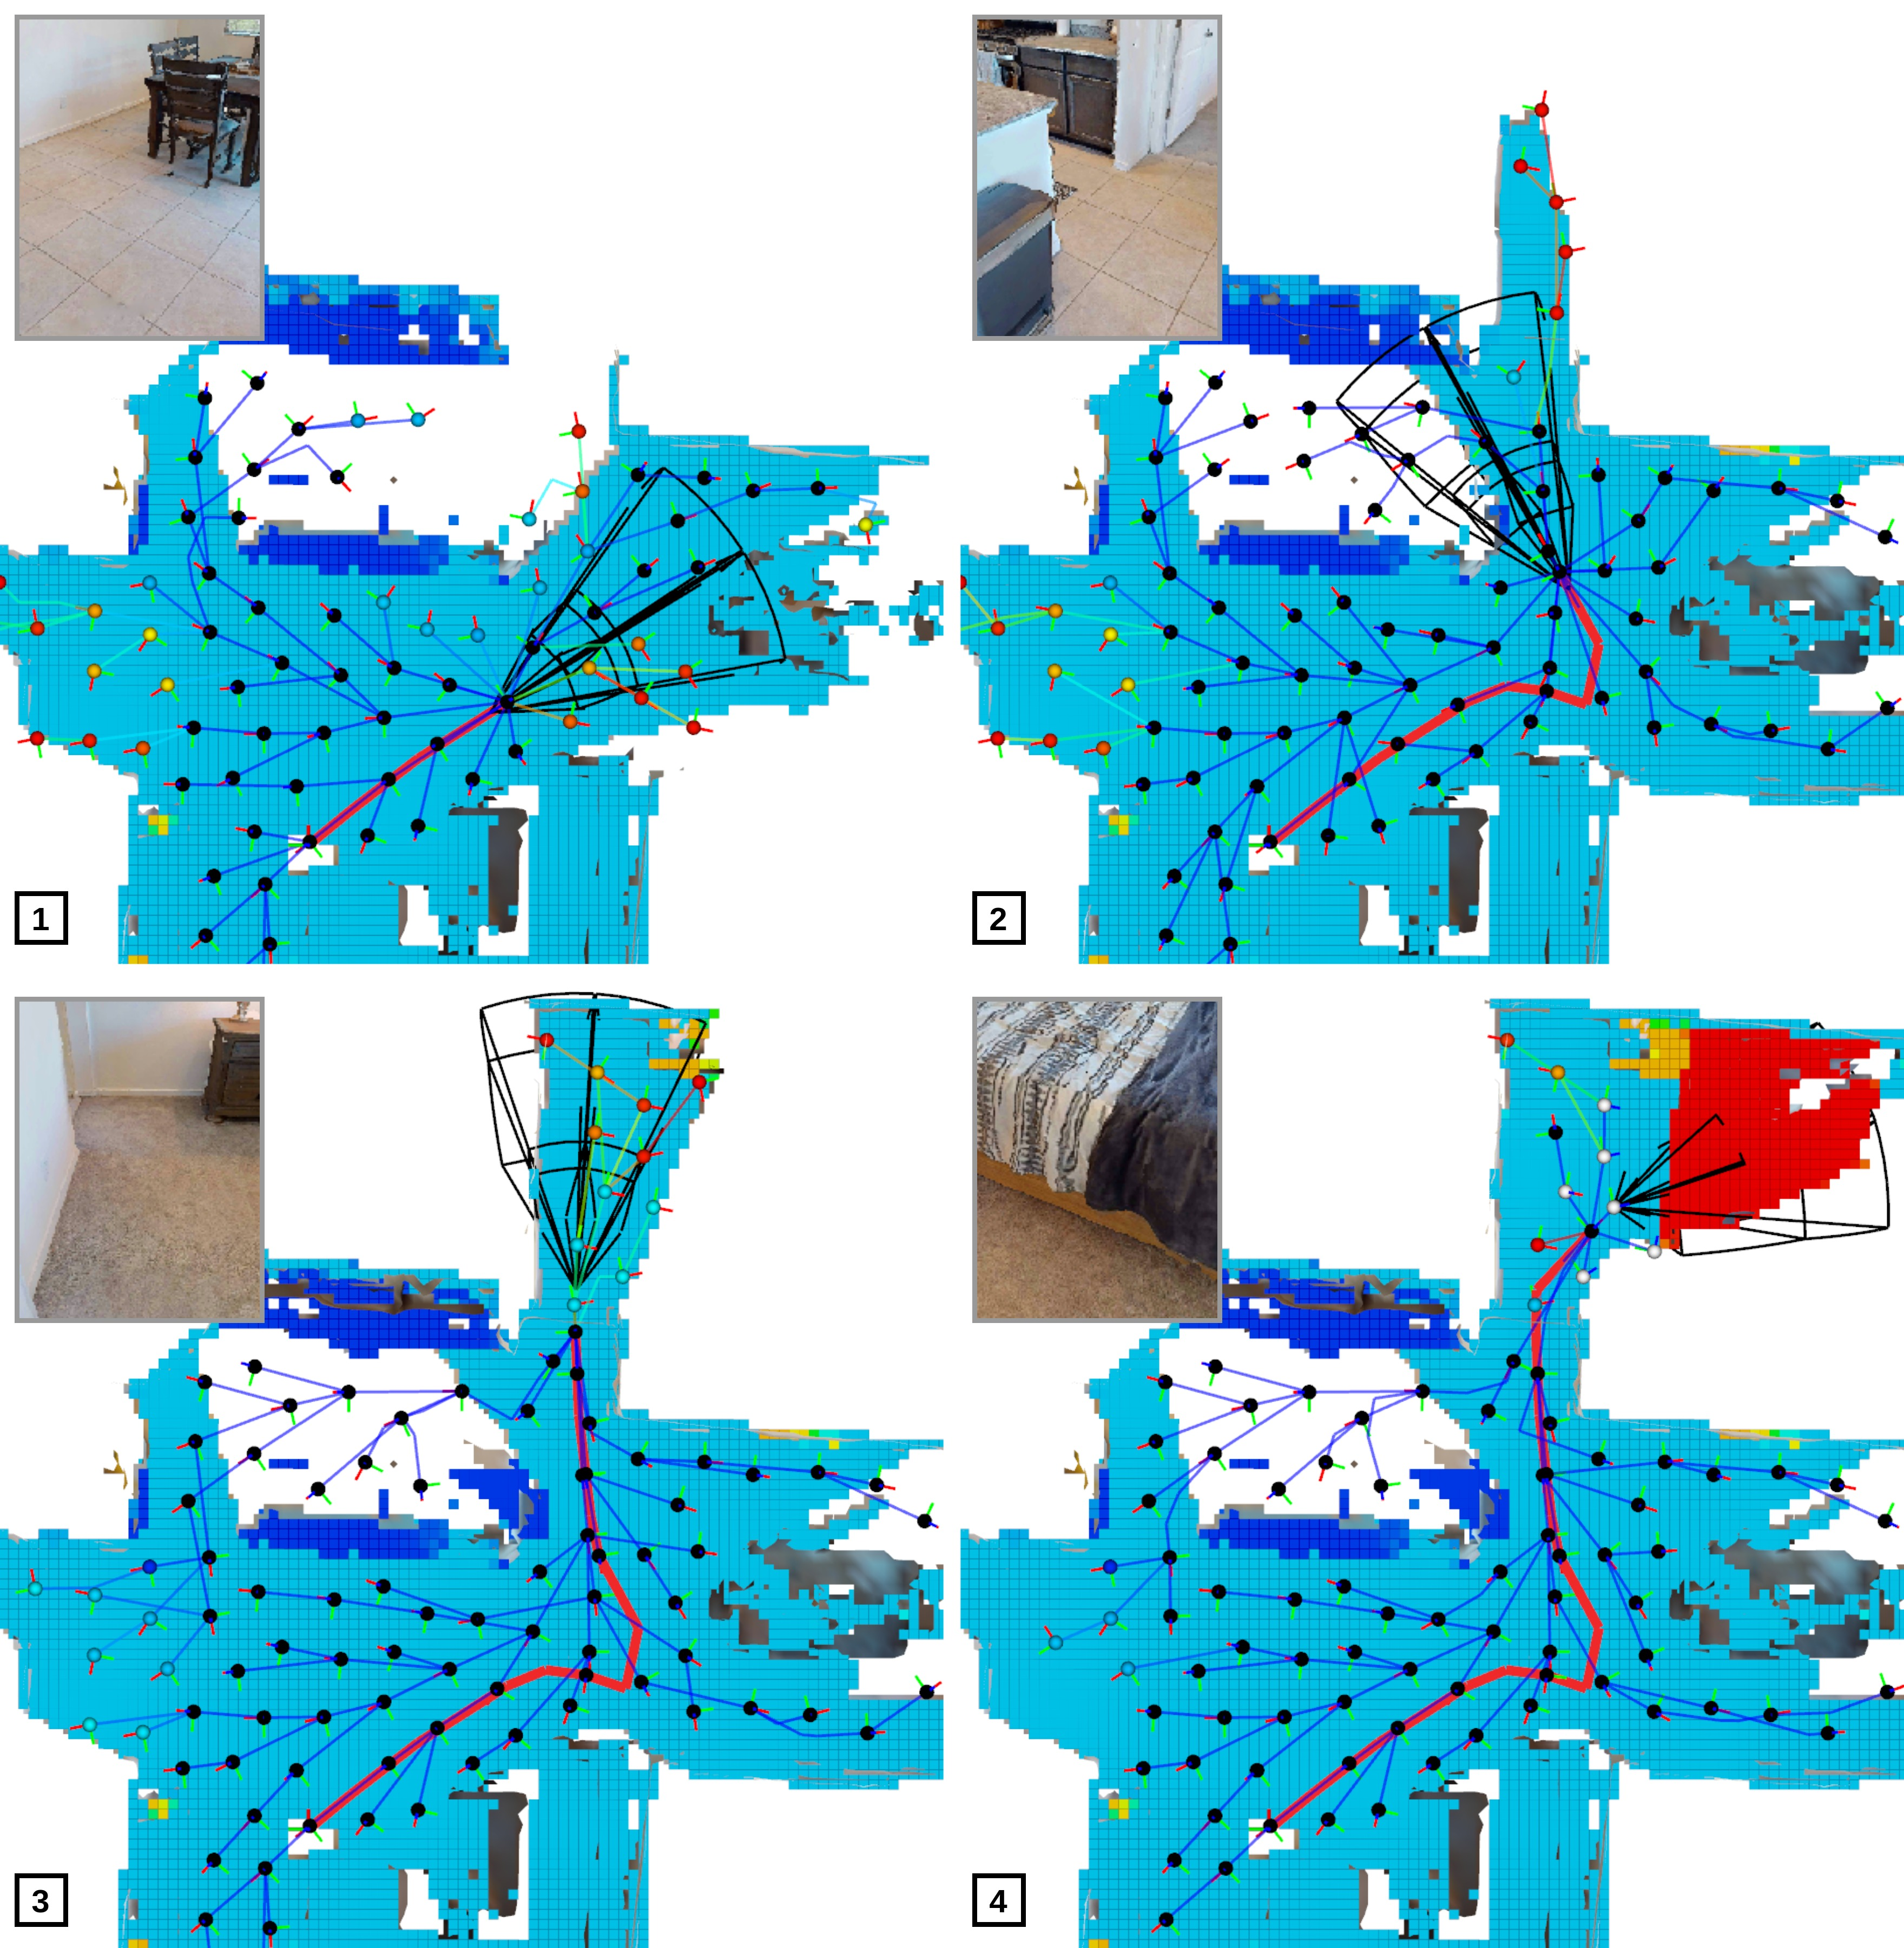}
    \caption{The robot finds a bed in the Habitat ObjectNav Challenge, in the same scene as the one in Fig.~\ref{fig:ippon-pipeline} and Fig.~\ref{fig:imagined-probability}. The visualization includes both the larger view frustum for gain evaluation and the smaller one for termination evaluation, alongside the RGB image. The map shown is a proximity map (identical to that in Fig.~\ref{fig:imagined-probability}). The nodes are color-coded: terminating nodes in white, minimally-exploring nodes in black, and the rest based on their gain -- from highest (red) to lowest (blue). In the second timestamp, nodes on the left and the top have comparable gains. However, by the third timestamp, after the robot identifies a chest of drawers at the top, the left nodes show a reduced gain relative to the top nodes.  The edges are similarly colored according to the gain-to-cost ratio ${G(P_n)} / {C(P_n)}$, as in Eq.~\ref{eq:node-selection}. The significantly higher gain-to-cost ratio at the top prompts the robot to explore nearby areas, ultimately leading it to terminate at a white terminating node.}
    \label{fig:find-bed}
\end{figure}

\begin{figure}[ht]
    \centering
    \begin{subfigure}{\textwidth}
        \includegraphics[width=\linewidth]{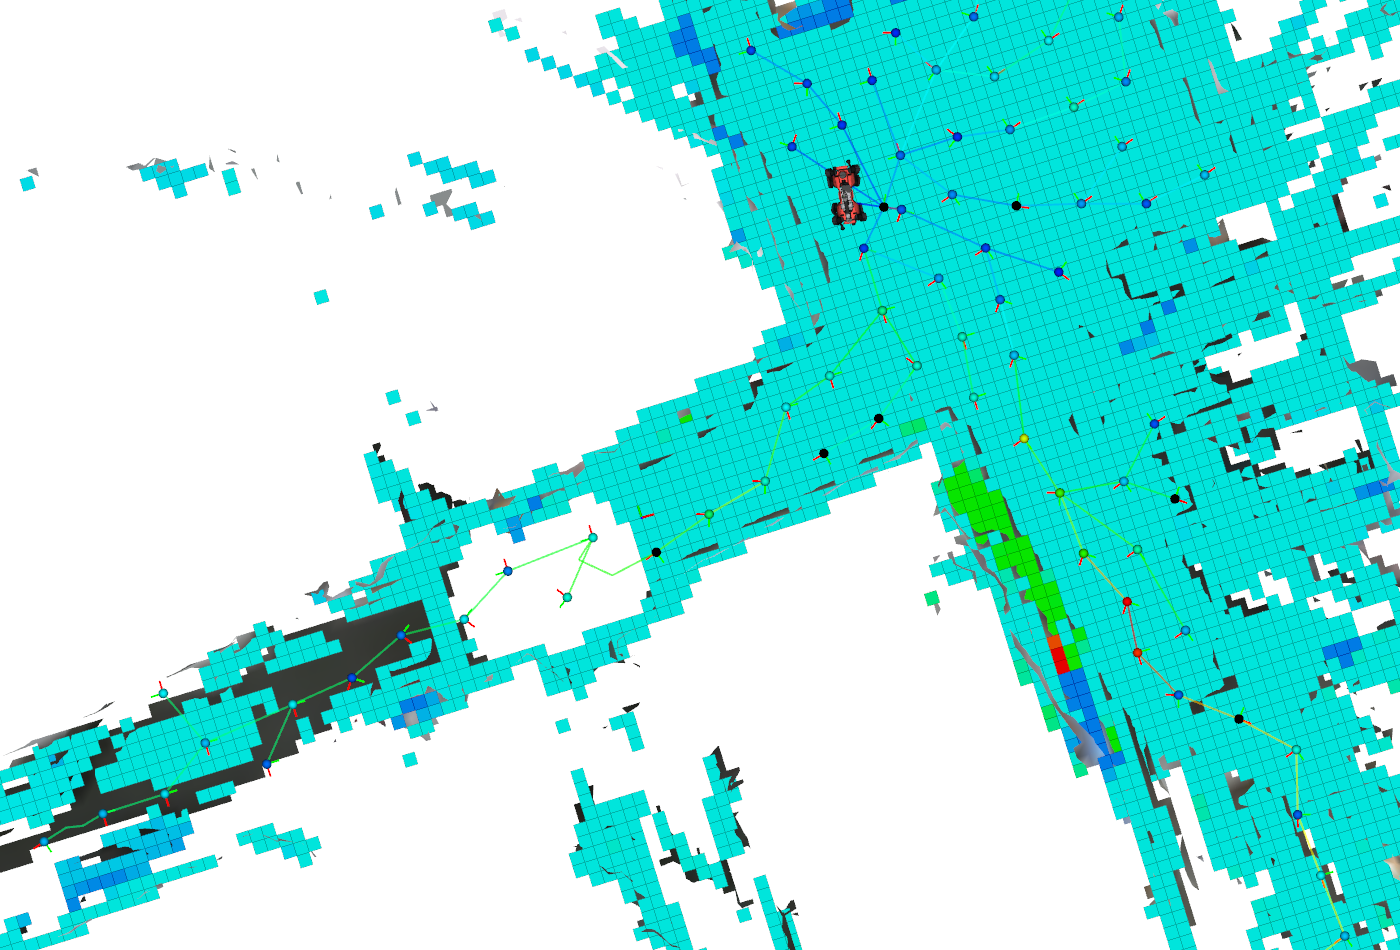}
        \caption{As the robot begins its navigation to find a microwave oven, the highest values and gains are identified near the microwave oven, indicated by the red voxels, nodes, and edges.}
        \label{fig:find-all-objects-microwave-oven}
    \end{subfigure}
    \begin{subfigure}{\textwidth}
        \includegraphics[width=\linewidth]{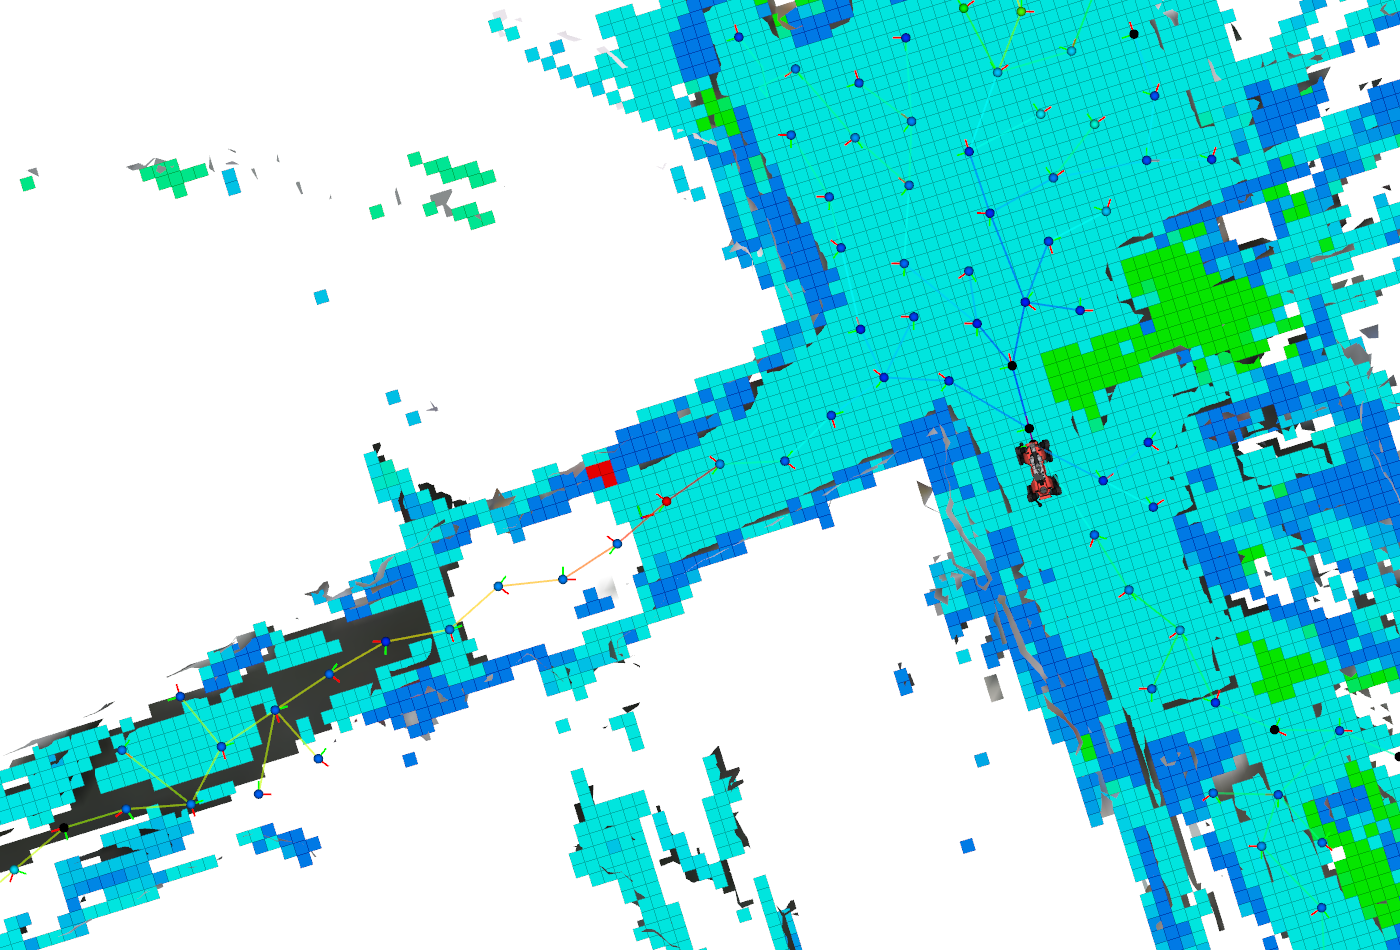}
        \caption{As the robot begins its navigation to find a plant, the highest values and gains are identified near the plant, indicated by the red voxels, node, and edges.}
        \label{fig:find-all-objects-plant}
    \end{subfigure}
    \caption{These illustrations show how a previously constructed common object map facilitates subsequent searches. The final trajectories for finding a microwave and a plant can be found in Fig.~\ref{fig:all-in-one}. The visualization follows the same scheme as in Fig.~\ref{fig:find-bed}.}
    \label{fig:find-all-objects-proximity-map}
\end{figure}

\begin{figure}[ht]
    \centering
    \includegraphics[width=\linewidth]{imgs/find_microwave_oven_long_distance_blurred.jpg}
    \caption{The robot navigates a challenging environment to locate a microwave oven, requiring it to traverse at least 30 meters and make a minimum of two turns.}
    \label{fig:find-microwave-oven-long-distance}
\end{figure}
